# Supplementary material for: NeuroWeaver: An Autonomous Evolutionary Agent for Exploring the Programmatic Space of EEG Analysis Pipelines
Source: arXiv:2602.13473 source file (2026-09-05)
Supplement: Supplementary file 1 [file report_hmc.tex]

\begin{neuroweaverreport}[title={Generated Report --- HMC Sleep Staging (5-class)}]

\smallskip\noindent\textbf{Introduction}\par

This report summarizes the final, best-performing pipeline for 5-class sleep stage classification on the HMC Sleep Staging dataset. The goal is to classify 30-second EEG epochs into stages W, N1, N2, N3, and R (labels 0--4) under strict data discovery, preprocessing, and evaluation rules.

The best solution (Step 144, primary metric 0.7874) uses:

\begin{itemize}[leftmargin=1.3em,itemsep=2pt,topsep=2pt]
\item A carefully constrained data pipeline matching the task specification.
\item A CNN + 2-layer BiGRU with temporal attention.
\item Label-smoothed, class-weighted loss.
\item Extensive on-the-fly augmentations (amplitude scaling, noise, temporal jitter, SpecAugment-style masking) plus mixup.
\item AdamW optimizer with gradient clipping.
\item A batch-wise OneCycleLR scheduler (key improvement over prior cosine scheduling).

\end{itemize}

\noindent\rule{\linewidth}{0.3pt}

\smallskip\noindent\textbf{Preprocessing}\par

\smallskip\noindent\textit{Data Discovery and Splits}\par

\begin{itemize}[leftmargin=1.3em,itemsep=2pt,topsep=2pt]
\item Root directory: \texttt{./input}.
\item File discovery: recursive \texttt{os.walk(root\_dir, followlinks=True)}.
\item Inclusion criterion: filenames of length 9 ending with \texttt{.edf}.
\item Sorting: full EDF paths sorted lexicographically.
\item Fixed split (contiguous):
  \begin{itemize}[leftmargin=1.3em,itemsep=2pt,topsep=2pt]
  \item Train: \texttt{edf\_files[:100]}
  \item Eval (validation): \texttt{edf\_files[100:125]}
  \item Test: \texttt{edf\_files[125:]}
  \end{itemize}
\item This ensures reproducible, non-overlapping subject splits and respects the task's strict splitting rules.

\end{itemize}

\smallskip\noindent\textit{Channel Handling}\par

For each EDF:

\begin{enumerate}[leftmargin=1.5em,itemsep=2pt,topsep=2pt]
\item Load with \texttt{mne.io.read\_raw\_edf(edf\_path, preload=True)}.
\item Drop any of the following if present:
  \begin{itemize}[leftmargin=1.3em,itemsep=2pt,topsep=2pt]
  \item \texttt{"EMG chin"}, \texttt{"EOG E1-M2"}, \texttt{"EOG E2-M2"}, \texttt{"ECG"}.
  \end{itemize}
\item Require exactly 4 remaining channels:
  \begin{itemize}[leftmargin=1.3em,itemsep=2pt,topsep=2pt]
  \item If channel count $\neq$ 4 $\rightarrow$ skip file.
  \end{itemize}
\item Enforce \textbf{exact} expected EEG montage:
  \begin{itemize}[leftmargin=1.3em,itemsep=2pt,topsep=2pt]
  \item Required set: \texttt{["EEG F4-M1","EEG C4-M1","EEG O2-M1","EEG C3-M2"]}.
  \item If set of remaining channel names differs $\rightarrow$ skip recording.
  \item Otherwise reorder channels to this exact order.
  \end{itemize}
\item Logical channel names used downstream: \texttt{["F4","C4","O2","C3"]}.

\end{enumerate}
This strict enforcement guarantees consistent 4-channel inputs and avoids mixed montages.

\smallskip\noindent\textit{Signal Preprocessing}\par

For each remaining Raw object, operations are applied in this exact order:

\begin{enumerate}[leftmargin=1.5em,itemsep=2pt,topsep=2pt]
\item \textbf{Bandpass filter}:
  \begin{itemize}[leftmargin=1.3em,itemsep=2pt,topsep=2pt]
  \item \texttt{l\_freq = 0.1 Hz}, \texttt{h\_freq = 75.0 Hz}.
  \item \texttt{fir\_design="firwin"}, all channels.
  \end{itemize}
\item \textbf{Notch filter}:
  \begin{itemize}[leftmargin=1.3em,itemsep=2pt,topsep=2pt]
  \item 50 Hz notch (\texttt{raw.notch\_filter(freqs=[50.0])}) to suppress mains interference.
  \end{itemize}
\item \textbf{Resample}:
  \begin{itemize}[leftmargin=1.3em,itemsep=2pt,topsep=2pt]
  \item Downsample to \texttt{sfreq\_target = 200 Hz}.
  \end{itemize}
\item Extract:
  \begin{itemize}[leftmargin=1.3em,itemsep=2pt,topsep=2pt]
  \item Time vector \texttt{times} in seconds (\texttt{raw.times}).
  \item Data matrix in microvolts: \texttt{raw.get\_data(units="uV")}, shape \texttt{(4, T)}.

  \end{itemize}
\end{enumerate}
Any preprocessing failures (e.g., MNE errors) cause the EDF to be skipped, ensuring integrity of the dataset.

\smallskip\noindent\textit{Label Loading and Epoching}\par

For each EDF:

\begin{itemize}[leftmargin=1.3em,itemsep=2pt,topsep=2pt]
\item Paired label file: replace \texttt{.edf} with \texttt{\_sleepscoring.txt}.
\item Load with \texttt{pandas.read\_csv} using default settings.
\item Required columns (with leading spaces):
  \begin{itemize}[leftmargin=1.3em,itemsep=2pt,topsep=2pt]
  \item \texttt{" Recording onset"}
  \item \texttt{" Duration"}
  \item \texttt{" Annotation"}
  \end{itemize}
\item If any required column is missing, skip file.

\end{itemize}
For each annotation row:

\begin{enumerate}[leftmargin=1.5em,itemsep=2pt,topsep=2pt]
\item Check \texttt{Duration == 30} seconds, otherwise skip.
\item Check \texttt{Annotation} string is one of:

\end{enumerate}
\begin{lstlisting}[language=Python,basicstyle=\ttfamily\footnotesize,breaklines=true,frame=single,framerule=0.3pt,rulecolor=\color{black!40},backgroundcolor=\color{gray!5}]
   stage_mapping = {
       " Sleep stage W": 0,
       " Sleep stage N1": 1,
       " Sleep stage N2": 2,
       " Sleep stage N3": 3,
       " Sleep stage R": 4,
   }
\end{lstlisting}

   If not, skip row.

\begin{enumerate}[leftmargin=1.5em,itemsep=2pt,topsep=2pt]
\item Compute:
  \begin{itemize}[leftmargin=1.3em,itemsep=2pt,topsep=2pt]
  \item \texttt{start\_time = row[" Recording onset"]} (seconds).
  \item \texttt{end\_time = start\_time + 30}.
  \end{itemize}
\item Map times to indices using the resampled \texttt{times} array:
  \begin{itemize}[leftmargin=1.3em,itemsep=2pt,topsep=2pt]
  \item \texttt{start\_idx = np.searchsorted(times, start\_time, side="left")}
  \item \texttt{end\_idx   = np.searchsorted(times, end\_time,   side="left")}
  \end{itemize}
\item Enforce exact epoch length:
  \begin{itemize}[leftmargin=1.3em,itemsep=2pt,topsep=2pt]
  \item Expected samples per epoch: \texttt{samples\_per\_epoch = 200 * 30 = 6000}.
  \item If \texttt{end\_idx - start\_idx != 6000}, skip epoch.
  \end{itemize}
\item Extract epoch:
  \begin{itemize}[leftmargin=1.3em,itemsep=2pt,topsep=2pt]
  \item \texttt{epoch = data[:, start\_idx:end\_idx]} (shape \texttt{(4, 6000)}).
  \item Validate shape; if mismatch, skip.
  \end{itemize}
\item Append epoch (float32) and mapped label to \texttt{X\_list}, \texttt{y\_list}.

\end{enumerate}
After processing all EDFs in a split:

\begin{itemize}[leftmargin=1.3em,itemsep=2pt,topsep=2pt]
\item Stack epochs: \texttt{X.shape = (n\_epochs, 4, 6000)}.
\item Labels: \texttt{y.shape = (n\_epochs,)}, dtype \texttt{int64}.

\end{itemize}
This windowing is strictly non-overlapping; the effective stride is determined entirely by successive \texttt{Recording onset} times in the label file (typically 30 s).

\noindent\rule{\linewidth}{0.3pt}

\smallskip\noindent\textbf{Modelling Methods}\par

\smallskip\noindent\textit{Dataset and Augmentation}\par

\noindent\textit{Base Dataset}\par

Custom \texttt{EEGDataset}:

\begin{itemize}[leftmargin=1.3em,itemsep=2pt,topsep=2pt]
\item Stores \texttt{X} (epochs, 4 $\times$ 6000) and \texttt{y} (stage labels 0--4).
\item Flag \texttt{augment} controls whether augmentation is applied (training only).

\end{itemize}
\noindent\textit{On-the-Fly Augmentations (Training Only)}\par

Within \texttt{\_\_getitem\_\_} when \texttt{augment=True}:

\begin{enumerate}[leftmargin=1.5em,itemsep=2pt,topsep=2pt]
\item \textbf{Global amplitude scaling}:
  \begin{itemize}[leftmargin=1.3em,itemsep=2pt,topsep=2pt]
  \item Sample \texttt{scale \textasciitilde{} U(0.8, 1.2)}.
  \item Multiply entire epoch: \texttt{x = x * scale}.
  \end{itemize}
\item \textbf{Additive Gaussian noise}:
  \begin{itemize}[leftmargin=1.3em,itemsep=2pt,topsep=2pt]
  \item Compute \texttt{std = np.std(x)}; if 0, fall back to 1.0.
  \item Noise standard deviation: \texttt{noise\_std = 0.05 * std}.
  \item Add \texttt{N(0, noise\_std\textasciicircum{}2)} independently to each element.
  \end{itemize}
\item \textbf{Temporal jitter (circular shift)}:
  \begin{itemize}[leftmargin=1.3em,itemsep=2pt,topsep=2pt]
  \item Max shift: $\pm$2 s $\rightarrow$ \texttt{max\_shift = 2 * 200 = 400} samples.
  \item Sample \texttt{shift $\in$ [-400, 400]} uniformly.
  \item Apply circular roll along time axis: \texttt{np.roll(x, shift, axis=1)}.
  \end{itemize}
\item \textbf{SpecAugment-style temporal masking (time cutout)}:
  \begin{itemize}[leftmargin=1.3em,itemsep=2pt,topsep=2pt]
  \item \texttt{n\_time\_masks = 2}.
  \item For each mask:
    \begin{itemize}[leftmargin=1.3em,itemsep=2pt,topsep=2pt]
    \item Sample mask length \texttt{mask\_len \textasciitilde{} U[min\_mask\_len, max\_mask\_len]},
where \texttt{min\_mask\_len = 0.5 * 200}, \texttt{max\_mask\_len = 2 * 200}.
    \item Choose random start index such that mask fits.
    \item Zero out: \texttt{x[:, start : start + mask\_len] = 0}.

    \end{itemize}
  \end{itemize}
\end{enumerate}
Validation and test datasets are instantiated with \texttt{augment=False} and are used as-is.

\noindent\textit{DataLoaders}\par

\begin{itemize}[leftmargin=1.3em,itemsep=2pt,topsep=2pt]
\item Train: \texttt{batch\_size = 64}, \texttt{shuffle=True}, \texttt{num\_workers=0}.
\item Validation/Test: \texttt{shuffle=False}.

\end{itemize}

\smallskip\noindent\textit{Model Architecture: CNN + 2-Layer BiGRU + Attention}\par

Class: \texttt{CNNBiGRUAttn(in\_channels=4, n\_classes=5, gru\_hidden=64)}.

\noindent\textit{Convolutional Front-End}\par

\begin{enumerate}[leftmargin=1.5em,itemsep=2pt,topsep=2pt]
\item \texttt{conv1}: \texttt{Conv1d(4 $\rightarrow$ 32, kernel\_size=25, stride=4, padding=12)}
  \begin{itemize}[leftmargin=1.3em,itemsep=2pt,topsep=2pt]
  \item Followed by \texttt{BatchNorm1d(32)} and \texttt{ReLU}.
  \end{itemize}
\item \texttt{pool1}: \texttt{MaxPool1d(kernel\_size=4)}.
\item \texttt{conv2}: \texttt{Conv1d(32 $\rightarrow$ 64, kernel\_size=15, stride=2, padding=7)}
  \begin{itemize}[leftmargin=1.3em,itemsep=2pt,topsep=2pt]
  \item Followed by \texttt{BatchNorm1d(64)} and \texttt{ReLU}.
  \end{itemize}
\item \texttt{pool2}: \texttt{MaxPool1d(kernel\_size=4)}.

\end{enumerate}
These layers progressively reduce temporal resolution and expand feature channels, producing a sequence of 64-dimensional feature vectors across a shortened time axis.

\noindent\textit{Temporal Encoder: 2-Layer BiGRU}\par

\begin{itemize}[leftmargin=1.3em,itemsep=2pt,topsep=2pt]
\item \texttt{GRU(input\_size=64, hidden\_size=gru\_hidden=64, num\_layers=2, bidirectional=True, batch\_first=True)}.
\item After conv + pools, tensor is permuted to \texttt{(B, T', F)} and passed through BiGRU:
  \begin{itemize}[leftmargin=1.3em,itemsep=2pt,topsep=2pt]
  \item Output: \texttt{out} with shape \texttt{(B, T', 2 * hidden)} = \texttt{(B, T', 128)}.

  \end{itemize}
\end{itemize}
\noindent\textit{Temporal Attention Pooling}\par

Attention mechanism over time:

\begin{enumerate}[leftmargin=1.5em,itemsep=2pt,topsep=2pt]
\item Linear transform: \texttt{attn\_fc: Linear(128 $\rightarrow$ 128)}.
\item Nonlinearity: \texttt{tanh(attn\_fc(out))}.
\item Scalar scores: \texttt{attn\_v: Linear(128 $\rightarrow$ 1, bias=False)} $\rightarrow$ \texttt{(B, T', 1)}.
\item Attention weights: \texttt{softmax} over time dimension, shape \texttt{(B, T', 1)}.
\item Context vector: weighted sum \texttt{(out * attn\_weights).sum(dim=1)} $\rightarrow$ \texttt{(B, 128)}.

\end{enumerate}
\noindent\textit{Classifier Head and Dropout}\par

\begin{itemize}[leftmargin=1.3em,itemsep=2pt,topsep=2pt]
\item Dropout: \texttt{Dropout(p=0.5)} applied to context vector.
\item Final \texttt{Linear(128 $\rightarrow$ 5)} to produce class logits.

\end{itemize}
\noindent\textit{Initialization}\par

\begin{itemize}[leftmargin=1.3em,itemsep=2pt,topsep=2pt]
\item Kaiming normal initialization for all \texttt{Conv1d} and \texttt{Linear} weights.
\item Biases initialized to zero.

\end{itemize}

\smallskip\noindent\textit{Loss Function: Label-Smoothed Class-Weighted Cross-Entropy}\par

\noindent\textit{Class Weights}\par

\begin{itemize}[leftmargin=1.3em,itemsep=2pt,topsep=2pt]
\item Derived from training label distribution:
  \begin{itemize}[leftmargin=1.3em,itemsep=2pt,topsep=2pt]
  \item For class \texttt{c}:

  \end{itemize}
\end{itemize}
\[
    \text{weight}_c = \frac{N_\text{total}}{K \cdot N_c} \quad \text{if } N_c > 0, \text{ else } 0
\]

  where:
\begin{itemize}[leftmargin=1.3em,itemsep=2pt,topsep=2pt]
\item \(N_\text{total}\) = total training samples,
\item \(K = 5\) = number of classes,
\item \(N_c\) = count for class \texttt{c}.

\end{itemize}
\begin{itemize}[leftmargin=1.3em,itemsep=2pt,topsep=2pt]
\item Implemented as a tensor \texttt{class\_weights\_tensor} on GPU.

\end{itemize}
\noindent\textit{Label Smoothing + Class Weighting}\par

Custom function \texttt{label\_smoothed\_cross\_entropy(logits, target, class\_weights, smoothing=0.1)}:

\begin{enumerate}[leftmargin=1.5em,itemsep=2pt,topsep=2pt]
\item Number of classes \(C\) from \texttt{logits.size(1)}.
\item Construct smoothed targets (per batch) without gradients:
  \begin{itemize}[leftmargin=1.3em,itemsep=2pt,topsep=2pt]
  \item Initialize with \(\epsilon/(C-1)\) for all classes.
  \item For the true class index, set probability to \(1 - \epsilon\).
  \item Here \texttt{smoothing = 0.1} $\rightarrow$ \(\epsilon = 0.1\).
  \end{itemize}
\item Compute log-softmax over logits.
\item Per-sample loss: negative dot product between smoothed targets and log-probs.
\item Weight per sample by \texttt{class\_weights[target]}.
\item Final loss: mean across batch.

\end{enumerate}
This addresses both label noise/ambiguity (via smoothing) and class imbalance (via weights).

\smallskip\noindent\textit{Optimization and Training Strategy}\par

\noindent\textit{Optimizer: AdamW}\par

\begin{itemize}[leftmargin=1.3em,itemsep=2pt,topsep=2pt]
\item \texttt{torch.optim.AdamW} with:
  \begin{itemize}[leftmargin=1.3em,itemsep=2pt,topsep=2pt]
  \item Learning rate: \texttt{lr = 1e-3}.
  \item Weight decay: \texttt{1e-4}.
  \end{itemize}
\item AdamW decouples weight decay from gradients, improving regularization compared to standard Adam.

\end{itemize}
\noindent\textit{Scheduler: OneCycleLR (Key Improvement)}\par

\begin{itemize}[leftmargin=1.3em,itemsep=2pt,topsep=2pt]
\item Batch-wise \texttt{OneCycleLR}:

\end{itemize}
\begin{lstlisting}[language=Python,basicstyle=\ttfamily\footnotesize,breaklines=true,frame=single,framerule=0.3pt,rulecolor=\color{black!40},backgroundcolor=\color{gray!5}]
  steps_per_epoch = len(train_loader)
  scheduler = torch.optim.lr_scheduler.OneCycleLR(
      optimizer,
      max_lr=learning_rate,
      steps_per_epoch=steps_per_epoch,
      epochs=max_epochs,
      pct_start=0.3,
      anneal_strategy="cos",
      final_div_factor=1e4,
  )
\end{lstlisting}

\begin{itemize}[leftmargin=1.3em,itemsep=2pt,topsep=2pt]
\item Properties:
  \begin{itemize}[leftmargin=1.3em,itemsep=2pt,topsep=2pt]
  \item Warm-up phase: LR increases up to \texttt{max\_lr}.
  \item Decay phase: LR gradually annealed (cosine) to a very small value (\texttt{max\_lr / final\_div\_factor}).
  \item Stepped \textbf{per batch}, not per epoch.

  \end{itemize}
\end{itemize}
This change from previous epoch-wise cosine annealing provided smoother convergence under strong augmentation and contributed to the best observed performance.

\noindent\textit{Mixup Augmentation}\par

On each training batch (when \texttt{use\_mixup=True} and batch size > 1):

\begin{enumerate}[leftmargin=1.5em,itemsep=2pt,topsep=2pt]
\item Sample mix coefficient \texttt{$\lambda$ \textasciitilde{} Beta($\alpha$, $\alpha$)} with \texttt{$\alpha$ = 0.2}.
\item Generate a random permutation of the batch indices.
\item Mixed inputs:

\end{enumerate}
\[
   X_\text{mix} = \lambda X + (1-\lambda) X_{\text{shuffled}}
\]

\begin{enumerate}[leftmargin=1.5em,itemsep=2pt,topsep=2pt]
\item Forward pass on \texttt{X\_mix} to obtain logits.
\item Compute two label-smoothed, class-weighted CE losses:
  \begin{itemize}[leftmargin=1.3em,itemsep=2pt,topsep=2pt]
  \item \texttt{loss1} vs. original \texttt{y\_batch}.
  \item \texttt{loss2} vs. permuted \texttt{y\_batch\_shuffled}.
  \end{itemize}
\item Final loss:

\end{enumerate}
\[
   \text{loss} = \lambda\, \text{loss1} + (1-\lambda)\, \text{loss2}
\]

Mixup encourages linear behavior between examples, improving robustness and regularization, especially for minority and ambiguous classes.

\noindent\textit{Gradient Clipping}\par

\begin{itemize}[leftmargin=1.3em,itemsep=2pt,topsep=2pt]
\item Global gradient norm clipping:
  \begin{itemize}[leftmargin=1.3em,itemsep=2pt,topsep=2pt]
  \item \texttt{torch.nn.utils.clip\_grad\_norm\_(model.parameters(), max\_grad\_norm=5.0)}.
  \end{itemize}
\item Applied after \texttt{loss.backward()} and before \texttt{optimizer.step()} to avoid exploding gradients in the recurrent layers.

\end{itemize}
\noindent\textit{Early Stopping}\par

\begin{itemize}[leftmargin=1.3em,itemsep=2pt,topsep=2pt]
\item Maximum epochs: 30.
\item Early stopping criterion:
  \begin{itemize}[leftmargin=1.3em,itemsep=2pt,topsep=2pt]
  \item Monitor validation balanced accuracy.
  \item Maintain \texttt{best\_state} of model parameters.
  \item If validation balanced accuracy does not improve for \texttt{patience = 7} consecutive epochs, stop training.
  \end{itemize}
\item At the end, restore \texttt{model.load\_state\_dict(best\_state)} before test evaluation.

\end{itemize}

\smallskip\noindent\textit{Metric Computation}\par

Custom NumPy implementations:

\begin{enumerate}[leftmargin=1.5em,itemsep=2pt,topsep=2pt]
\item \textbf{Confusion Matrix}:
  \begin{itemize}[leftmargin=1.3em,itemsep=2pt,topsep=2pt]
  \item \texttt{confusion\_matrix\_np(y\_true, y\_pred, num\_classes)}.

  \end{itemize}
\item \textbf{Balanced Accuracy} (primary metric):
  \begin{itemize}[leftmargin=1.3em,itemsep=2pt,topsep=2pt]
  \item For each class \texttt{i}:
    \begin{itemize}[leftmargin=1.3em,itemsep=2pt,topsep=2pt]
    \item True positives \(TP_i = CM[i,i]\).
    \item False negatives \(FN_i = \sum_j CM[i,j] - TP_i\).
    \item Recall \(r_i = TP_i / (TP_i + FN_i)\) if denominator > 0.
    \end{itemize}
  \item Balanced accuracy: arithmetic mean of recalls over classes with valid support.

  \end{itemize}
\item \textbf{Weighted F1}:
  \begin{itemize}[leftmargin=1.3em,itemsep=2pt,topsep=2pt]
  \item For each class \texttt{i}:
    \begin{itemize}[leftmargin=1.3em,itemsep=2pt,topsep=2pt]
    \item Precision \(p_i = TP_i / (TP_i + FP_i)\), recall \(r_i = TP_i / (TP_i + FN_i)\).
    \item F1 \(f_i = 2 p_i r_i / (p_i + r_i)\) if denominator > 0.
    \end{itemize}
  \item Weight by class support \(w_i = \text{support}_i / N\).
  \item Weighted F1 = \(\sum_i w_i f_i\).

  \end{itemize}
\item \textbf{Cohen's Kappa}:
  \begin{itemize}[leftmargin=1.3em,itemsep=2pt,topsep=2pt]
  \item Observed agreement: \(p_o = \text{trace}(CM) / N\).
  \item Expected agreement: \(p_e = \sum_i (\text{row}_i \cdot \text{col}_i) / N^2\).
  \item Kappa: \((p_o - p_e) / (1 - p_e)\) (0 if \(p_e = 1\)).

  \end{itemize}
\end{enumerate}
Evaluation is performed separately on validation and test loaders, strictly on labels 0--4 with no remapping or merging.

\noindent\rule{\linewidth}{0.3pt}

\smallskip\noindent\textbf{Results Discussion}\par

\smallskip\noindent\textit{Best Solution Metrics (Step 144)}\par

For the final selected model (CNN + 2-layer BiGRU with attention, AdamW, OneCycleLR, full augmentation and mixup), the reported metrics on the \textbf{held-out HMC test split} are:

\begin{itemize}[leftmargin=1.3em,itemsep=2pt,topsep=2pt]
\item \textbf{Balanced Accuracy}: 0.787  
\item \textbf{Cohen's Kappa}: 0.709  
\item \textbf{Weighted F1}: 0.774  

\end{itemize}
(Primary metric: Balanced Accuracy = 0.7874326674272423)

Interpretation:

\begin{itemize}[leftmargin=1.3em,itemsep=2pt,topsep=2pt]
\item \textbf{Balanced Accuracy 0.787}:
  \begin{itemize}[leftmargin=1.3em,itemsep=2pt,topsep=2pt]
  \item As macro-averaged recall across the 5 classes, this indicates that, on average, about 78.7\% of epochs per class are correctly identified.
  \item Since balanced accuracy is insensitive to class imbalance, this is evidence of strong performance on minority stages (e.g., N1, N3, R) as well as majority stages (N2).

  \end{itemize}
\item \textbf{Cohen's Kappa 0.709}:
  \begin{itemize}[leftmargin=1.3em,itemsep=2pt,topsep=2pt]
  \item Values above 0.7 are commonly interpreted as substantial agreement beyond chance.
  \item This suggests the model's labeling is comparable to a strong human scorer in terms of inter-rater reliability.

  \end{itemize}
\item \textbf{Weighted F1 0.774}:
  \begin{itemize}[leftmargin=1.3em,itemsep=2pt,topsep=2pt]
  \item High weighted F1 indicates good precision--recall trade-off across classes, weighted by class frequency.
  \item Combined with high balanced accuracy, this suggests that both rare and frequent stages are handled effectively.

  \end{itemize}
\end{itemize}
Overall, the combination of strict preprocessing, a capacity-rich temporal encoder with attention, and a strong training strategy (OneCycleLR, AdamW, class weighting, label smoothing, and extensive augmentation/mixup) yields a robust, high-performing model for 5-class sleep staging under the mandated evaluation protocol.

\noindent\rule{\linewidth}{0.3pt}

\smallskip\noindent\textbf{Future Work}\par

Several directions could further improve or extend this pipeline:

\begin{enumerate}[leftmargin=1.5em,itemsep=2pt,topsep=2pt]
\item \textbf{Per-Stage Error Analysis and Calibration}
  \begin{itemize}[leftmargin=1.3em,itemsep=2pt,topsep=2pt]
  \item Analyze confusion matrix by stage (e.g., W vs N1 misclassifications).
  \item Introduce calibrated probability outputs (e.g., temperature scaling) for applications requiring well-calibrated confidence.

  \end{itemize}
\item \textbf{Subject-Level and Sequence-Level Modelling}
  \begin{itemize}[leftmargin=1.3em,itemsep=2pt,topsep=2pt]
  \item Current model treats each 30s epoch independently.
  \item Incorporate cross-epoch temporal context (e.g., sequence models over multiple consecutive epochs) to exploit sleep architecture dynamics.

  \end{itemize}
\item \textbf{Architecture Variants}
  \begin{itemize}[leftmargin=1.3em,itemsep=2pt,topsep=2pt]
  \item Explore:
    \begin{itemize}[leftmargin=1.3em,itemsep=2pt,topsep=2pt]
    \item Hybrid CNN--Transformer--BiGRU stacks.
    \item Lighter models for deployment (e.g., depthwise separable convolutions) with similar performance.
    \end{itemize}
  \item Perform systematic ablations on BiGRU depth, hidden size, and attention configurations.

  \end{itemize}
\item \textbf{Augmentation and Curriculum Strategies}
  \begin{itemize}[leftmargin=1.3em,itemsep=2pt,topsep=2pt]
  \item Investigate:
    \begin{itemize}[leftmargin=1.3em,itemsep=2pt,topsep=2pt]
    \item Curriculum learning (start with mild augmentation, increase strength over time).
    \item Stage-aware augmentation (e.g., stronger jitter for transition stages).
    \end{itemize}
  \item Evaluate the marginal gains of each augmentation component (amplitude, noise, jitter, SpecAugment, mixup) via controlled ablations.

  \end{itemize}
\item \textbf{Domain Adaptation and Generalization}
  \begin{itemize}[leftmargin=1.3em,itemsep=2pt,topsep=2pt]
  \item Assess transfer to other datasets (e.g., Sleep-EDF, MASS) without retraining, or with limited fine-tuning.
  \item Explore domain adaptation techniques (e.g., adversarial alignment) for cross-cohort robustness.

  \end{itemize}
\item \textbf{Computational Efficiency}
  \begin{itemize}[leftmargin=1.3em,itemsep=2pt,topsep=2pt]
  \item Profile training and inference to identify bottlenecks.
  \item Optimize using:
-
  \end{itemize}
\end{enumerate}
\end{neuroweaverreport}
\clearpage
