# Supplementary material for: NeuroWeaver: An Autonomous Evolutionary Agent for Exploring the Programmatic Space of EEG Analysis Pipelines
Source: arXiv:2602.13473 source file (2026-09-05)
Supplement: Supplementary file 2 [file report_seed.tex]

\begin{neuroweaverreport}[title={Generated Report --- SEED Emotion Classification (3-class)}]

\smallskip\noindent\textbf{Introduction}\par

This work addresses 3-class emotion classification (Positive, Neutral, Negative) on the SEED EEG dataset using strict, trial-based splits. The best-performing configuration combines:

\begin{itemize}[leftmargin=1.3em,itemsep=2pt,topsep=2pt]
\item A Temporal ResNet-style 1D CNN with squeeze-and-excitation (SE) channel attention and temporal attention pooling  
\item AdamW optimization with class weighting and label smoothing  
\item On-the-fly channel-dropout augmentation during training  
\item Exponential Moving Average (EMA) of model parameters for validation and test evaluation  
\item No temporal masking or jitter in the final best run

\end{itemize}
The goal is robust window-level emotion recognition from 62-channel, 4 s EEG windows under a standardized preprocessing and evaluation protocol.

\noindent\rule{\linewidth}{0.3pt}

\smallskip\noindent\textbf{Preprocessing}\par

\smallskip\noindent\textit{Data loading and inclusion criteria}\par

\begin{itemize}[leftmargin=1.3em,itemsep=2pt,topsep=2pt]
\item Root: \texttt{./input}, recursively scan for \texttt{.cnt} files.
\item File selection: filenames with a trailing session ID in \texttt{\{1,2,3\}} are treated as valid SEED sessions.
\item Loading: \texttt{mne.io.read\_raw\_cnt(preload=True, data\_format='int32')}.

\end{itemize}

\smallskip\noindent\textit{Channel handling}\par

\begin{itemize}[leftmargin=1.3em,itemsep=2pt,topsep=2pt]
\item Drop channels if present: \texttt{['M1', 'M2', 'VEO', 'HEO']} and \texttt{'ECG'} (if present).
\item No further channel reordering or dropping.
\item Require exactly 62 remaining channels; otherwise skip the file.

\end{itemize}

\smallskip\noindent\textit{Signal preprocessing}\par

Applied in this order to each accepted recording:

\begin{enumerate}[leftmargin=1.5em,itemsep=2pt,topsep=2pt]
\item \textbf{Bandpass filter}: 0.1--75 Hz (FIR, \texttt{firwin}).
\item \textbf{Notch filter}: 50 Hz.
\item \textbf{Resampling}: 200 Hz (from original SEED sampling rate).
\item \textbf{Units}: \texttt{raw.get\_data(units='uV')} to get microvolt-level data.
\item \textbf{No additional normalization}: no per-channel z-scoring, no global scaling.

\end{enumerate}

\smallskip\noindent\textit{Trial segmentation}\par

Fixed SEED trial timings (seconds):

\begin{itemize}[leftmargin=1.3em,itemsep=2pt,topsep=2pt]
\item \texttt{trialStartTime = [24, 289, 550, 782, 1049, 1260, 1483, 1747, 1993, 2283, 2550, 2812, 3072, 3332, 3598]}
\item \texttt{trialEndTime   = [264, 526, 757, 1023, 1235, 1458, 1722, 1967, 2259, 2525, 2788, 3046, 3308, 3573, 3806]}
\item Labels per trial: \texttt{['H','N','S','S','N','H','S','N','H','H','N','S','N','H','S']}

\end{itemize}
Label mapping (fixed, never remapped):

\begin{itemize}[leftmargin=1.3em,itemsep=2pt,topsep=2pt]
\item Positive (H) $\rightarrow$ 0  
\item Neutral  (N) $\rightarrow$ 1  
\item Negative (S) $\rightarrow$ 2  

\end{itemize}
For each trial \texttt{i} (0-based index):

\begin{itemize}[leftmargin=1.3em,itemsep=2pt,topsep=2pt]
\item Convert start/end seconds to samples at 200 Hz:  
\texttt{start\_samp = int(trialStartTime[i]*200)}, \texttt{end\_samp = int(trialEndTime[i]*200)}.
\item If \texttt{end\_samp > n\_times} (recording too short), skip that trial.

\end{itemize}

\smallskip\noindent\textit{Windowing}\par

Per valid trial segment:

\begin{itemize}[leftmargin=1.3em,itemsep=2pt,topsep=2pt]
\item Window length: 4.0 s = 800 samples.
\item Stride: 800 samples (non-overlapping).
\item Number of windows: \texttt{n\_windows = floor(T\_trial / 800)}. Any remainder \texttt{< 800} dropped.
\item Each window has shape \texttt{(62, 800)} and inherits the parent trial's integer label.

\end{itemize}

\smallskip\noindent\textit{Dataset splitting}\par

Splits are \textbf{trial-index based within each recording}:

\begin{itemize}[leftmargin=1.3em,itemsep=2pt,topsep=2pt]
\item Trials 1--9  (indices 0--8)   $\rightarrow$ TRAIN
\item Trials 10--12 (indices 9--11) $\rightarrow$ VAL
\item Trials 13--15 (indices 12--14)$\rightarrow$ TEST

\end{itemize}
For each \texttt{.cnt} file, windows are assigned to train/val/test according to its own trial indices, then concatenated across all recordings to form global TRAIN/VAL/TEST sets. No subject-wise or file-wise splitting is used; only trial-wise.

\noindent\rule{\linewidth}{0.3pt}

\smallskip\noindent\textbf{Modelling Methods}\par

\smallskip\noindent\textit{Overview of best solution}\par

The best-performing configuration (Step 163, primary metric 0.6278) uses:

\begin{itemize}[leftmargin=1.3em,itemsep=2pt,topsep=2pt]
\item \textbf{Backbone}: TemporalResNet1D with SE channel attention + temporal attention pooling.
\item \textbf{Loss}: class-weighted cross-entropy with label smoothing.
\item \textbf{Optimizer}: AdamW with weight decay.
\item \textbf{Regularization}:
  \begin{itemize}[leftmargin=1.3em,itemsep=2pt,topsep=2pt]
  \item Channel-dropout augmentation on training windows.
  \item Standard dropout in the classifier.
  \item EMA of parameters for evaluation.
  \end{itemize}
\item \textbf{No temporal masking/jitter} in the final best run (these had been explored and disabled before Step 163).

\end{itemize}

\smallskip\noindent\textit{Dataset and augmentation}\par

\noindent\textit{EEGDataset}\par

\begin{itemize}[leftmargin=1.3em,itemsep=2pt,topsep=2pt]
\item Underlying arrays: \texttt{X $\in$ $\mathbb{R}$\textasciicircum{}\{N$\times$C$\times$T\}}, \texttt{y $\in$ \{0,1,2\}\textasciicircum{}N}.
\item For training:
  \begin{itemize}[leftmargin=1.3em,itemsep=2pt,topsep=2pt]
  \item \texttt{augment=True}, \texttt{channel\_dropout\_p=0.1}.
  \item For each window:
    \begin{itemize}[leftmargin=1.3em,itemsep=2pt,topsep=2pt]
    \item Sample Bernoulli mask per channel with keep probability \texttt{1 - p}.
    \item Ensure at least one channel is kept.
    \item Multiply \texttt{(C, T)} by \texttt{(C, 1)} mask $\rightarrow$ random subset of channels zeroed.
    \end{itemize}
  \end{itemize}
\item For validation/test:
  \begin{itemize}[leftmargin=1.3em,itemsep=2pt,topsep=2pt]
  \item \texttt{augment=False}, \texttt{channel\_dropout\_p=0.0} (no augmentation).

  \end{itemize}
\end{itemize}
Data loaders:

\begin{itemize}[leftmargin=1.3em,itemsep=2pt,topsep=2pt]
\item Batch size: 128.
\item Training: shuffle = True.
\item Val/Test: shuffle = False.

\end{itemize}

\smallskip\noindent\textit{TemporalResNet1D + SE + Temporal Attention}\par

The core model operates directly on \texttt{(batch, channels, time)} windows.

\noindent\textit{Convolutional feature extractor}\par

Layers (no explicit residual blocks here; ``ResNet-style'' refers mainly to depth and pooling):

\begin{enumerate}[leftmargin=1.5em,itemsep=2pt,topsep=2pt]
\item \textbf{Conv1}:  
  \begin{itemize}[leftmargin=1.3em,itemsep=2pt,topsep=2pt]
  \item Input channels: 62  
  \item Output channels: 64  
  \item Kernel: 7, padding: 3, bias: False  
  \item Followed by BatchNorm1d(64), ReLU, MaxPool1d(2)  
  \item Time: 800 $\rightarrow$ 400

  \end{itemize}
\item \textbf{Conv2}:  
  \begin{itemize}[leftmargin=1.3em,itemsep=2pt,topsep=2pt]
  \item In: 64, Out: 128, kernel: 7, padding: 3  
  \item BatchNorm1d(128), ReLU, MaxPool1d(2)  
  \item Time: 400 $\rightarrow$ 200

  \end{itemize}
\item \textbf{Conv3}:  
  \begin{itemize}[leftmargin=1.3em,itemsep=2pt,topsep=2pt]
  \item In: 128, Out: 256, kernel: 7, padding: 3  
  \item BatchNorm1d(256), ReLU  

  \end{itemize}
\item \textbf{SE Block} (SEBlock1D on 256 channels):  
  \begin{itemize}[leftmargin=1.3em,itemsep=2pt,topsep=2pt]
  \item Global average over time $\rightarrow$ \texttt{(B, 256)}  
  \item FC1: 256 $\rightarrow$ max(1, 256/16) = 16  
  \item ReLU  
  \item FC2: 16 $\rightarrow$ 256  
  \item Sigmoid $\rightarrow$ \texttt{(B, 256)} channel-wise weights  
  \item Rescale feature maps: \texttt{x * weights.view(B, 256, 1)}

  \end{itemize}
\item \textbf{Pool3}: MaxPool1d(2)  
  \begin{itemize}[leftmargin=1.3em,itemsep=2pt,topsep=2pt]
  \item Time: 200 $\rightarrow$ 100

  \end{itemize}
\end{enumerate}
Result: a feature map \texttt{(B, 256, 100)}.

\noindent\textit{Temporal Attention Pooling}\par

\texttt{TemporalAttentionPooling(in\_channels=256, hidden\_channels=64)}:

\begin{itemize}[leftmargin=1.3em,itemsep=2pt,topsep=2pt]
\item 1$\times$1 Conv: 256 $\rightarrow$ 64, Tanh nonlinearity.
\item 1$\times$1 Conv: 64 $\rightarrow$ 1 $\rightarrow$ logits \texttt{(B, 1, T)}.
\item Softmax over time $\rightarrow$ attention weights \texttt{(B, 1, T)}.
\item Weighted sum: \texttt{$\Sigma$\_t w\_t * x\_t} over time $\rightarrow$ context \texttt{(B, 256)}.

\end{itemize}
This replaces a fixed global pooling, allowing the model to emphasize temporally informative segments.

\noindent\textit{Classifier head}\par

\begin{itemize}[leftmargin=1.3em,itemsep=2pt,topsep=2pt]
\item Linear: 256 $\rightarrow$ 128
\item ReLU
\item Dropout(0.5)
\item Linear: 128 $\rightarrow$ 3 (class logits)

\end{itemize}

\smallskip\noindent\textit{Loss and class imbalance handling}\par

\noindent\textit{Class weighting}\par

\begin{itemize}[leftmargin=1.3em,itemsep=2pt,topsep=2pt]
\item Compute class counts on full training set: \texttt{counts[c]}.
\item Avoid zero counts by replacing zeros with 1.
\item Class weights:

\end{itemize}
\[
w_c = \frac{\sum_c \text{counts}[c]}{3 \cdot \text{counts}[c]}
\]

\begin{itemize}[leftmargin=1.3em,itemsep=2pt,topsep=2pt]
\item Used as \texttt{weight} argument in loss to counter class imbalance.

\end{itemize}
\noindent\textit{Label-smoothed cross-entropy}\par

Loss: \texttt{nn.CrossEntropyLoss(weight=class\_weights, label\_smoothing=0.1)}.

\begin{itemize}[leftmargin=1.3em,itemsep=2pt,topsep=2pt]
\item Hard integer labels remain \texttt{0,1,2}.
\item Label smoothing $\varepsilon$ = 0.1 modifies target distribution \texttt{y}:

  \begin{itemize}[leftmargin=1.3em,itemsep=2pt,topsep=2pt]
  \item Correct class: \texttt{1 - $\varepsilon$}  
  \item Other classes: \texttt{$\varepsilon$ / (K - 1)} with \texttt{K = 3}.

  \end{itemize}
\item This reduces overconfidence, especially helpful for noisy EEG emotion labels.

\end{itemize}

\smallskip\noindent\textit{Optimization and EMA}\par

\noindent\textit{Optimizer}\par

\begin{itemize}[leftmargin=1.3em,itemsep=2pt,topsep=2pt]
\item AdamW (\texttt{torch.optim.AdamW}) with:
  \begin{itemize}[leftmargin=1.3em,itemsep=2pt,topsep=2pt]
  \item Learning rate: \texttt{1e-3}
  \item Weight decay: \texttt{1e-2}

  \end{itemize}
\end{itemize}
Training setup:

\begin{itemize}[leftmargin=1.3em,itemsep=2pt,topsep=2pt]
\item Max epochs: 50.
\item Early stopping patience: 10 epochs (on validation balanced accuracy).
\item Device: GPU if available.

\end{itemize}
\noindent\textit{Exponential Moving Average (EMA)}\par

Two models:

\begin{itemize}[leftmargin=1.3em,itemsep=2pt,topsep=2pt]
\item \texttt{model}: trainable parameters updated by optimizer.
\item \texttt{ema\_model}: shadow copy updated after each optimizer step:

\end{itemize}
\[
\theta^{\text{EMA}} \leftarrow \text{decay} \cdot \theta^{\text{EMA}} + (1-\text{decay}) \cdot \theta
\]

\begin{itemize}[leftmargin=1.3em,itemsep=2pt,topsep=2pt]
\item Decay: 0.999.
\item \texttt{requires\_grad=False} for EMA parameters.

\end{itemize}
\textbf{Validation \& Test}:

\begin{itemize}[leftmargin=1.3em,itemsep=2pt,topsep=2pt]
\item Balanced accuracy for early stopping is computed using \texttt{ema\_model}.
\item Best EMA state (by validation balanced accuracy) is stored.
\item Final evaluation (VAL and TEST) uses this best \texttt{ema\_model}.

\end{itemize}

\smallskip\noindent\textit{Evaluation metrics}\par

For any dataloader:

\begin{enumerate}[leftmargin=1.5em,itemsep=2pt,topsep=2pt]
\item Forward pass with model in \texttt{eval()} mode.
\item Predicted labels: \texttt{argmax(logits, dim=1)}.
\item Compute on integer labels \{0,1,2\}:
  \begin{itemize}[leftmargin=1.3em,itemsep=2pt,topsep=2pt]
  \item \textbf{Balanced Accuracy} (macro-averaged recall across 3 classes).
  \item \textbf{Cohen's Kappa}.
  \item \textbf{Weighted F1} (class-support-weighted).

  \end{itemize}
\end{enumerate}
Balanced accuracy on TEST is the \textbf{primary metric} for model selection.

\noindent\rule{\linewidth}{0.3pt}

\smallskip\noindent\textbf{Results Discussion}\par

\smallskip\noindent\textit{Best configuration}\par

The \textbf{best-performing solution} is at \textbf{Step 163}, which:

\begin{itemize}[leftmargin=1.3em,itemsep=2pt,topsep=2pt]
\item Uses the TemporalResNet1D + SE + temporal attention backbone.
\item Uses AdamW + class-weighted label-smoothed cross-entropy.
\item Includes on-the-fly \textbf{channel-dropout} augmentation for training.
\item Maintains \textbf{EMA} of parameters.
\item \textbf{Disables SpecAugment-style temporal masking} (no zeroing of time segments).
\item Keeps all preprocessing, splitting, and metric computation as described above.

\end{itemize}

\smallskip\noindent\textit{Test-set performance (BEST SOLUTION)}\par

On the held-out SEED TEST split:

\begin{itemize}[leftmargin=1.3em,itemsep=2pt,topsep=2pt]
\item \textbf{Balanced Accuracy (primary metric)}: \textbf{0.6278}
\item \textbf{Cohen's Kappa}: \textbf{0.450}
\item \textbf{Weighted F1}: \textbf{0.631}

\end{itemize}
All metrics are computed directly on the integer labels:

\begin{itemize}[leftmargin=1.3em,itemsep=2pt,topsep=2pt]
\item 0: Positive (H)  
\item 1: Neutral (N)  
\item 2: Negative (S)

\end{itemize}
without any label remapping or smoothing at evaluation time.

\smallskip\noindent\textit{Interpretation}\par

\begin{itemize}[leftmargin=1.3em,itemsep=2pt,topsep=2pt]
\item \textbf{Balanced accuracy $\approx$ 0.628} is clearly above chance (1/3 $\approx$ 0.333) for 3-class classification, demonstrating substantial discriminative ability under a strict trial-based split.
\item \textbf{Cohen's Kappa $\approx$ 0.45} indicates moderate agreement beyond chance, suggesting that the model's predictions align reasonably well with human labels despite noisiness and inter-subject variability.
\item \textbf{Weighted F1 $\approx$ 0.631} shows that the model handles the class distribution reasonably, not overfitting heavily to the majority class.

\end{itemize}
The combination that appears crucial for this performance includes:

\begin{enumerate}[leftmargin=1.5em,itemsep=2pt,topsep=2pt]
\item \textbf{Rich temporal modeling} via long-kernel Conv1d layers and temporal attention pooling.
\item \textbf{SE channel attention} to emphasize informative electrodes/feature channels.
\item \textbf{AdamW with class weighting and label smoothing} to handle imbalance and noisy labels.
\item \textbf{Channel-dropout augmentation} to increase robustness to channel-specific artifacts.
\item \textbf{EMA of parameters} to smooth out stochastic optimization noise and improve generalization.
\item \textbf{Avoiding temporal masking} in the final best run, preserving potentially emotion-relevant brief transients.

\end{enumerate}
Ablation steps earlier in the journal show that:

\begin{itemize}[leftmargin=1.3em,itemsep=2pt,topsep=2pt]
\item Removing EMA or channel dropout generally reduced performance.
\item Temporal masking (time-masking) and aggressive jitter tended to slightly hurt macro recall on SEED in this setting.
\item Alternative backbones (e.g., pure EEGNet, simple TCN, some GRU-only designs) typically yielded lower balanced accuracy on the same protocol.

\end{itemize}
Thus, the Step 163 configuration represents a well-balanced tradeoff between model capacity, regularization, and data augmentation tailored to this dataset.

\noindent\rule{\linewidth}{0.3pt}

\smallskip\noindent\textbf{Future Work}\par

Several directions can extend or refine this approach:

\begin{enumerate}[leftmargin=1.5em,itemsep=2pt,topsep=2pt]
\item \textbf{Stronger subject/sequence modeling}
  \begin{itemize}[leftmargin=1.3em,itemsep=2pt,topsep=2pt]
  \item Investigate hierarchical models that aggregate multiple windows per trial or per subject, rather than independent window-level classification.
  \item Apply sequence models over window embeddings (e.g., Transformer over window-wise representations across a trial).

  \end{itemize}
\item \textbf{Domain adaptation and personalization}
  \begin{itemize}[leftmargin=1.3em,itemsep=2pt,topsep=2pt]
  \item Explore subject-adaptive layers or meta-learning to better handle inter-subject variability.
  \item Consider adversarial domain adaptation between subjects or sessions.

  \end{itemize}
\item \textbf{Improved temporal architectures}
  \begin{itemize}[leftmargin=1.3em,itemsep=2pt,topsep=2pt]
  \item Replace simple temporal attention pooling with multi-head self-attention or lightweight Transformers while preserving the current CNN+SE feature extractor.
  \item Introduce dilated convolutions in the best-performing TemporalResNet1D backbone (beyond what was already tested in other runs) in a more systematic grid.

  \end{itemize}
\item \textbf{Richer but targeted augmentations}
  \begin{itemize}[leftmargin=1.3em,itemsep=2pt,topsep=2pt]
  \item Carefully reintroduce temporal augmentations (small jitter, mild time masking) under tighter control:
    \begin{itemize}[leftmargin=1.3em,itemsep=2pt,topsep=2pt]
    \item Smaller masked fraction.
    \item Schedule-based probability (e.g., stronger early, weaker late).
    \end{itemize}
  \item Explore frequency-domain augmentations (band dropout, slight spectral warping) that preserve label semantics.

  \end{itemize}
\item \textbf{Calibration and uncertainty}
  \begin{itemize}[leftmargin=1.3em,itemsep=2pt,topsep=2pt]
  \item Analyze predictive uncertainty and calibration under label smoothing.
  \item Use confidence-aware decision rules or ensemble EMA variants.

  \end{itemize}
\item \textbf{Cross-dataset generalization}
  \begin{itemize}[leftmargin=1.3em,itemsep=2pt,topsep=2pt]
  \item Validate the preprocessing and TemporalResNet1D+SE+attention+EMA stack on other emotion EEG datasets (e.g., DEAP, MAHNOB-HCI) to test robustness and portability.

  \end{itemize}
\item \textbf{Interpretability}
  \begin{itemize}[leftmargin=1.3em,itemsep=2pt,topsep=2pt]
  \item Inspect learned SE channel weights and attention maps to identify:
    \begin{itemize}[leftmargin=1.3em,itemsep=2pt,topsep=2pt]
    \item Which electrodes and time segments are most informative.
    \end{itemize}
  \item Relate these to known neurophysiological correlates of emotion.

  \end{itemize}
\end{enumerate}
Systematic exploration along these lines is likely to further improve balanced accuracy and robustness beyond the current best of 0.6278 on the SEED test split.
\end{neuroweaverreport}
\clearpage
