# Supplementary material for: NeuroWeaver: An Autonomous Evolutionary Agent for Exploring the Programmatic Space of EEG Analysis Pipelines
Source: arXiv:2602.13473 source file (2026-09-05)
Supplement: Supplementary file 3 [file report_tuev.tex]

\begin{neuroweaverreport}[title={Generated Report --- TUEV Event Classification (6-class)}]

\smallskip\noindent\textbf{Introduction}\par

This report summarizes the final pipeline for 6-class EEG event classification on the TUH EEG Event Corpus (TUEV), adhering to the official \texttt{/train} and \texttt{/eval} directory protocol. The objective is to classify events into six classes (1=spsw, 2=gped, 3=pled, 4=eyem, 5=artf, 6=bckg) using subject-independent training/validation splits and reporting Balanced Accuracy (primary), Cohen's $\kappa$, and Weighted F1 on the held-out \texttt{/eval} test set.

The \textbf{best solution} (Step 184) achieves a \textbf{test Balanced Accuracy of 0.6365}, with a shallow 4-block ResNet1D backbone and a fully specified augmentation and optimization strategy. All other components of the data pipeline and training procedure remain consistent with earlier iterations, so performance gains can be attributed to the architectural change.

\noindent\rule{\linewidth}{0.3pt}

\smallskip\noindent\textbf{Preprocessing}\par

\smallskip\noindent\textit{Data loading and channel handling}\par

\begin{itemize}[leftmargin=1.3em,itemsep=2pt,topsep=2pt]
\item \textbf{Input structure}: 
  \begin{itemize}[leftmargin=1.3em,itemsep=2pt,topsep=2pt]
  \item Training recordings: \texttt{./input/train}
  \item Test recordings: \texttt{./input/eval}
  \end{itemize}
\item For each directory:
  \begin{itemize}[leftmargin=1.3em,itemsep=2pt,topsep=2pt]
  \item Traverse recursively, find \texttt{.edf} files.
  \item For each \texttt{.edf}, require a paired \texttt{.rec} with the same basename.

  \end{itemize}
\item \textbf{Patient ID}:
  \begin{itemize}[leftmargin=1.3em,itemsep=2pt,topsep=2pt]
  \item Extracted as the prefix of the EDF basename before the first underscore, e.g. \texttt{00000101\_s002\_t000.edf $\rightarrow$ patient\_id = "00000101"}.

  \end{itemize}
\item \textbf{Channel selection}:
  \begin{itemize}[leftmargin=1.3em,itemsep=2pt,topsep=2pt]
  \item Any recording is \textbf{skipped} unless it contains \textbf{all} of the following 23 EEG channels:
    \begin{enumerate}[leftmargin=1.5em,itemsep=2pt,topsep=2pt]
    \item EEG FP1-REF  
    \item EEG FP2-REF  
    \item EEG F3-REF  
    \item EEG F4-REF  
    \item EEG C3-REF  
    \item EEG C4-REF  
    \item EEG P3-REF  
    \item EEG P4-REF  
    \item EEG O1-REF  
    \item EEG O2-REF  
    \item EEG F7-REF  
    \item EEG F8-REF  
    \item EEG T3-REF  
    \item EEG T4-REF  
    \item EEG T5-REF  
    \item EEG T6-REF  
    \item EEG A1-REF  
    \item EEG A2-REF  
    \item EEG FZ-REF  
    \item EEG CZ-REF  
    \item EEG PZ-REF  
    \item EEG T1-REF  
    \item EEG T2-REF  
    \end{enumerate}
  \item MNE is used to \textbf{pick and reorder} channels to exactly this order.

  \end{itemize}
\end{itemize}

\smallskip\noindent\textit{Signal preprocessing}\par

For each valid EDF recording:

\begin{itemize}[leftmargin=1.3em,itemsep=2pt,topsep=2pt]
\item Load with \textbf{MNE} (\texttt{read\_raw\_edf(..., preload=True)}).
\item Apply filters:
  \begin{itemize}[leftmargin=1.3em,itemsep=2pt,topsep=2pt]
  \item \textbf{Bandpass}: 0.1--75 Hz (IIR).
  \item \textbf{Notch}: 60 Hz.
  \end{itemize}
\item \textbf{Resample} to 200 Hz using MNE (\texttt{raw.resample(200.0)}).
\item Obtain data:
  \begin{itemize}[leftmargin=1.3em,itemsep=2pt,topsep=2pt]
  \item \texttt{raw.get\_data(units="uV")} $\rightarrow$ \texttt{float32} array of shape \texttt{(23, N)}.
  \item \texttt{raw.times} $\rightarrow$ \texttt{float64} array of timestamps (seconds) of length \texttt{N}.
  \end{itemize}
\item No further normalization is applied; amplitudes are in microvolts as required.

\end{itemize}

\smallskip\noindent\textit{Event parsing}\par

For each \texttt{.rec} file:

\begin{itemize}[leftmargin=1.3em,itemsep=2pt,topsep=2pt]
\item Plain text, comma-separated, no header.
\item Each line:
  \begin{itemize}[leftmargin=1.3em,itemsep=2pt,topsep=2pt]
  \item \texttt{channel\_index, start\_time\_sec, stop\_time\_sec, label\_id}
  \end{itemize}
\item The pipeline:
  \begin{itemize}[leftmargin=1.3em,itemsep=2pt,topsep=2pt]
  \item Parses integer \texttt{channel\_index} (offending channel) but does \textbf{not} use it for modeling; classification is \textbf{per-segment} over all 23 channels.
  \item Uses \texttt{label\_id} as a 1..6 integer. Lines with invalid or out-of-range labels are discarded.
  \item Keeps all valid events; no de-duplication.

  \end{itemize}
\end{itemize}

\smallskip\noindent\textit{Event-centered segmentation with triple-signal semantics}\par

Target segment: \textbf{5 seconds} (1000 samples) per event.

Given:
\begin{itemize}[leftmargin=1.3em,itemsep=2pt,topsep=2pt]
\item Data: \texttt{data} of shape \texttt{(23, N)} at 200 Hz.
\item Time axis: \texttt{times} (length \texttt{N}).
\item For each event \texttt{(ch\_idx, start\_sec, stop\_sec, label\_id)}:

\item \textbf{Locate sample indices}:
  \begin{itemize}[leftmargin=1.3em,itemsep=2pt,topsep=2pt]
  \item \texttt{start\_idx = searchsorted(times, start\_sec, side="left")}
  \item \texttt{end\_idx   = searchsorted(times, stop\_sec, side="left")}
  \item Clip to \texttt{[0, N-1]} and enforce \texttt{end\_idx >= start\_idx}.

  \end{itemize}
\item \textbf{Extended triple-signal indexing}:
  \begin{itemize}[leftmargin=1.3em,itemsep=2pt,topsep=2pt]
  \item Let \texttt{offset = N}.
  \item Define:
    \begin{itemize}[leftmargin=1.3em,itemsep=2pt,topsep=2pt]
    \item \texttt{PRE\_SAMPLES = POST\_SAMPLES = 400} (2 s at 200 Hz).
    \item \texttt{left\_ext  = offset + start\_idx - PRE\_SAMPLES}
    \item \texttt{right\_ext = offset + end\_idx   + POST\_SAMPLES}
    \end{itemize}
  \item Construct index vector:
    \begin{itemize}[leftmargin=1.3em,itemsep=2pt,topsep=2pt]
    \item \texttt{idx\_ext = np.arange(left\_ext, right\_ext, dtype=np.int64)}
    \item Modular wrap into \texttt{[0, N)}:
      \begin{itemize}[leftmargin=1.3em,itemsep=2pt,topsep=2pt]
      \item \texttt{idx\_mod = idx\_ext \% N}
      \end{itemize}
    \end{itemize}
  \item Extract segment:
    \begin{itemize}[leftmargin=1.3em,itemsep=2pt,topsep=2pt]
    \item \texttt{seg = data[:, idx\_mod]} $\rightarrow$ \texttt{(23, seg\_len)}
    \end{itemize}
  \item Enforce \textbf{fixed length}: if \texttt{seg.shape[1] != 1000}, discard this event (rare, due to inconsistent annotation spans).

  \end{itemize}
\item \textbf{Storage format}:
  \begin{itemize}[leftmargin=1.3em,itemsep=2pt,topsep=2pt]
  \item Segments stored as \texttt{float16} arrays for memory efficiency.
  \item Labels stored as \texttt{int64} in \{1,\textbackslash{}ldots\{\},6\}.

  \end{itemize}
\end{itemize}
This implementation is mathematically equivalent to the specified ``3N'' triple-concatenation semantics but avoids actually materializing a 3N array, which is important for memory scalability.

\smallskip\noindent\textit{Dataset construction and splitting}\par

\begin{itemize}[leftmargin=1.3em,itemsep=2pt,topsep=2pt]
\item Enumerate EDF/REC pairs in \texttt{./input/train}.
\item Derive the set of \textbf{unique patient IDs}.
\item Use \texttt{RandomState(SEED=4523)} to:
  \begin{itemize}[leftmargin=1.3em,itemsep=2pt,topsep=2pt]
  \item Permute patient IDs.
  \item Assign \textbf{80\% to training} and \textbf{20\% to validation}.
  \end{itemize}
\item Build three disjoint segment sets:
  \begin{itemize}[leftmargin=1.3em,itemsep=2pt,topsep=2pt]
  \item \textbf{Train}: segments from \texttt{/train} recordings whose patient ID $\in$ training set.
  \item \textbf{Validation}: segments from \texttt{/train} recordings whose patient ID $\in$ validation set.
  \item \textbf{Test}: all segments from \texttt{/eval}.
  \end{itemize}
\item Final arrays:
  \begin{itemize}[leftmargin=1.3em,itemsep=2pt,topsep=2pt]
  \item \texttt{X\_train, X\_val, X\_test}: \texttt{(N\_split, 23, 1000)} \texttt{float16}.
  \item \texttt{y\_train, y\_val, y\_test}: \texttt{(N\_split,)} \texttt{int64} labels in [1..6].

  \end{itemize}
\end{itemize}
The split is strictly subject-independent; no patient appears in more than one split.

\noindent\rule{\linewidth}{0.3pt}

\smallskip\noindent\textbf{Modelling Methods}\par

\smallskip\noindent\textit{Dataset wrapper and augmentations}\par

\texttt{EEGEventDataset} wraps \texttt{(X, y)} arrays:

\begin{itemize}[leftmargin=1.3em,itemsep=2pt,topsep=2pt]
\item \texttt{\_\_len\_\_}: number of segments.
\item \texttt{\_\_getitem\_\_(idx)}:
  \begin{itemize}[leftmargin=1.3em,itemsep=2pt,topsep=2pt]
  \item Loads \texttt{x = X[idx].astype(np.float32)} with shape \texttt{(23, 1000)}.
  \item Converts \texttt{y} from \texttt{[1..6]} to \texttt{[0..5]} for PyTorch CE (\texttt{y\_idx = y-1}).
  \item \textbf{Temporal jitter} (train only):
    \begin{itemize}[leftmargin=1.3em,itemsep=2pt,topsep=2pt]
    \item For training datasets, apply circular time shift:
      \begin{itemize}[leftmargin=1.3em,itemsep=2pt,topsep=2pt]
      \item Random \texttt{shift $\in$ [-100, 100]} samples ($\pm$0.5 s at 200 Hz).
      \item Implemented via \texttt{np.roll(x, shift=shift, axis=1)}.

      \end{itemize}
    \end{itemize}
  \end{itemize}
\end{itemize}
No augmentation is applied to validation or test data.

\smallskip\noindent\textit{Sampling and class weighting}\par

To address strong label imbalance:

\begin{enumerate}[leftmargin=1.5em,itemsep=2pt,topsep=2pt]
\item \textbf{Class weights for loss}:
  \begin{itemize}[leftmargin=1.3em,itemsep=2pt,topsep=2pt]
  \item For labels in \{1,\textbackslash{}ldots\{\},6\}:
    \begin{itemize}[leftmargin=1.3em,itemsep=2pt,topsep=2pt]
    \item Count per class in \texttt{y\_train}.
    \item Compute inverse-frequency weights:
      \begin{itemize}[leftmargin=1.3em,itemsep=2pt,topsep=2pt]
      \item \texttt{inv\_c = 1 / count\_c}
      \item Normalize: \texttt{weights = inv\_c / mean(inv\_c)}
      \end{itemize}
    \end{itemize}
  \item Pass as \texttt{weight=class\_weights} to \texttt{nn.CrossEntropyLoss}.

  \end{itemize}
\item \textbf{Class-balanced sampler}:
  \begin{itemize}[leftmargin=1.3em,itemsep=2pt,topsep=2pt]
  \item Recompute counts and inverse frequencies.
  \item Assign each training sample a weight: \texttt{weight[y\_train[i] - 1]}.
  \item Use \texttt{WeightedRandomSampler(weights=sample\_weights, num\_samples=len(sample\_weights), replacement=True)}.
  \item This yields mini-batches with a more balanced class composition, while preserving the original distribution in validation/test.

  \end{itemize}
\end{enumerate}

\smallskip\noindent\textit{Backbone architecture: 4-block 1D ResNet (ResNetEEG1D)}\par

The best solution uses a \textbf{shallow 4-block 1D ResNet} over time, with a single residual block per stage and an internal MaxPool inside each block.

\noindent\textit{ResBlock1D}\par

\begin{itemize}[leftmargin=1.3em,itemsep=2pt,topsep=2pt]
\item Two 1D convolutions with a residual connection and a trailing pool:

\end{itemize}
\begin{lstlisting}[basicstyle=\ttfamily\footnotesize,breaklines=true,frame=single,framerule=0.3pt,rulecolor=\color{black!40},backgroundcolor=\color{gray!5}]
  Conv1d(in_ch $\rightarrow$ out_ch, kernel=7, stride=stride, padding=3)
  BatchNorm1d
  ReLU
  Conv1d(out_ch $\rightarrow$ out_ch, kernel=7, stride=1, padding=3)
  BatchNorm1d
  + optional 1$\times$1 Conv1d + BN for downsampling when stride>1 or channel change
  ReLU
  + MaxPool1d(2) at the end of each block (`pool=True`)
\end{lstlisting}

\begin{itemize}[leftmargin=1.3em,itemsep=2pt,topsep=2pt]
\item Expansion = 1.

\end{itemize}
\noindent\textit{ResNetEEG1D}\par

Configuration:

\begin{itemize}[leftmargin=1.3em,itemsep=2pt,topsep=2pt]
\item \textbf{Input}: \texttt{(B, 23, 1000)}.

\item \textbf{Stem}:
  \begin{itemize}[leftmargin=1.3em,itemsep=2pt,topsep=2pt]
  \item \texttt{Conv1d(23 $\rightarrow$ 64, kernel=7, stride=1, padding=3)}
  \item \texttt{BatchNorm1d(64)}
  \item \texttt{ReLU}
  \item Temporal size: \texttt{1000 $\rightarrow$ 1000} (no pooling in stem).

  \end{itemize}
\item \textbf{Residual blocks} (4 single \texttt{ResBlock1D} modules, each with internal \texttt{MaxPool1d(2)}):

  \begin{enumerate}[leftmargin=1.5em,itemsep=2pt,topsep=2pt]
  \item \textbf{block1}: \texttt{ResBlock1D(64, 64, kernel=7, stride=1, pool=True)} $\rightarrow$ time \texttt{1000 $\rightarrow$ 500}.
  \item \textbf{block2}: \texttt{ResBlock1D(64, 128, kernel=7, stride=1, pool=True)} $\rightarrow$ time \texttt{500 $\rightarrow$ 250}.
  \item \textbf{block3}: \texttt{ResBlock1D(128, 128, kernel=7, stride=1, pool=True)} $\rightarrow$ time \texttt{250 $\rightarrow$ 125}.
  \item \textbf{block4}: \texttt{ResBlock1D(128, 256, kernel=7, stride=1, pool=True)} $\rightarrow$ time \texttt{125 $\rightarrow$ 62}.

  \end{enumerate}
\item \textbf{Head}:
  \begin{itemize}[leftmargin=1.3em,itemsep=2pt,topsep=2pt]
  \item \texttt{AdaptiveAvgPool1d(1)} $\rightarrow$ collapse time dimension $\rightarrow$ \texttt{(B, 256)}.
  \item \texttt{Linear(256 $\rightarrow$ 6)} logits.

  \end{itemize}
\end{itemize}
This shallow stack of four single residual blocks keeps the model lightweight (a few million parameters) while still providing four levels of multi-scale temporal abstraction over the 5-second window.

\smallskip\noindent\textit{Loss, optimizer, and learning-rate schedule}\par

\begin{itemize}[leftmargin=1.3em,itemsep=2pt,topsep=2pt]
\item \textbf{Loss}: \texttt{nn.CrossEntropyLoss(weight=class\_weights)} with labels in \texttt{[0..5]}.
  \begin{itemize}[leftmargin=1.3em,itemsep=2pt,topsep=2pt]
  \item No label smoothing; class imbalance handled by explicit weights and a class-balanced sampler.
  \end{itemize}
\item \textbf{Optimizer}: \texttt{Adam} with:
  \begin{itemize}[leftmargin=1.3em,itemsep=2pt,topsep=2pt]
  \item Initial learning rate: \texttt{LR = 1e-3}.
  \end{itemize}
\item \textbf{LR Schedule}: \texttt{CosineAnnealingWarmRestarts}:
  \begin{itemize}[leftmargin=1.3em,itemsep=2pt,topsep=2pt]
  \item \texttt{T\_0 = 10}, \texttt{T\_mult = 2}, \texttt{eta\_min = 1e-5}.
  \item Stepped \textbf{once per epoch} after validation.
  \end{itemize}
\item \textbf{Training regimen}:
  \begin{itemize}[leftmargin=1.3em,itemsep=2pt,topsep=2pt]
  \item \texttt{MAX\_EPOCHS = 30} (no early stopping; the full schedule is run).
  \item \texttt{BATCH\_SIZE = 64}.
  \item \texttt{NUM\_WORKERS = 2} for data loading.
  \item \texttt{pin\_memory = True} for faster device transfers.

  \end{itemize}
\end{itemize}
Mixup-style sample mixing was explored during the search but is not used in this final pipeline; class imbalance is addressed solely via class weighting and the weighted sampler.

\smallskip\noindent\textit{Training and evaluation loop}\par

\begin{itemize}[leftmargin=1.3em,itemsep=2pt,topsep=2pt]
\item \textbf{Best-state tracking}:
  \begin{itemize}[leftmargin=1.3em,itemsep=2pt,topsep=2pt]
  \item Monitor \textbf{validation balanced accuracy} after each epoch.
  \item Track \texttt{best\_val\_bal\_acc} and save the model state dict whenever it improves.
  \item Train for the full \texttt{MAX\_EPOCHS} schedule and reload the best state for evaluation.

  \end{itemize}
\item \textbf{Evaluation}:
  \begin{itemize}[leftmargin=1.3em,itemsep=2pt,topsep=2pt]
  \item For any split (val or test):
    \begin{itemize}[leftmargin=1.3em,itemsep=2pt,topsep=2pt]
    \item Use \texttt{DataLoader} with \texttt{shuffle=False}.
    \item Predict class via \texttt{argmax(logits, dim=1)} on \texttt{[0..5]}, then +1 to map back to \texttt{[1..6]}.
    \end{itemize}
  \item Metrics:
    \begin{itemize}[leftmargin=1.3em,itemsep=2pt,topsep=2pt]
    \item \textbf{Balanced Accuracy} (macro recall) over six classes.
    \item \textbf{Cohen's Kappa}.
    \item \textbf{Weighted F1} (sklearn \texttt{average="weighted"}).
    \end{itemize}
  \item The \textbf{primary metric} is test \textbf{Balanced Accuracy} on \texttt{/eval}.

  \end{itemize}
\end{itemize}

\noindent\rule{\linewidth}{0.3pt}

\smallskip\noindent\textbf{Results Discussion}\par

The \textbf{best solution} (Step 184) reports the following final metrics on the official TUEV \texttt{/eval} test set:

\begin{itemize}[leftmargin=1.3em,itemsep=2pt,topsep=2pt]
\item \textbf{Test Balanced Accuracy (primary)}: \textbf{0.6365}
\item \textbf{Test Cohen's Kappa}: \textbf{0.3491}
\item \textbf{Test Weighted F1}: \textbf{0.6122}

\end{itemize}
These values are obtained after:

\begin{itemize}[leftmargin=1.3em,itemsep=2pt,topsep=2pt]
\item Full MNE preprocessing (0.1--75 Hz, 60 Hz notch, resample to 200 Hz, $\mu$V).
\item Strict 23-channel enforcement and ordering.
\item Event-centered segmentation with triple-signal semantics.
\item Subject-wise 80/20 train/validation split (seed 4523).
\item Training with:
  \begin{itemize}[leftmargin=1.3em,itemsep=2pt,topsep=2pt]
  \item Shallow \textbf{ResNetEEG1D} backbone (4 single residual blocks at 64 / 128 / 128 / 256 channels).
  \item \textbf{Temporal jitter} ($\pm$0.5 s).
  \item \textbf{Class-balanced sampling} via \texttt{WeightedRandomSampler}.
  \item \textbf{Class-weighted cross-entropy} (no label smoothing, no mixup).
  \item \textbf{Cosine-annealing LR with warm restarts} ($T_0 = 10$, $T_{\text{mult}} = 2$).
  \item Best-state tracking on \textbf{validation balanced accuracy} across the full 30-epoch schedule.

  \end{itemize}
\end{itemize}

\smallskip\noindent\textit{Interpretation}\par

\begin{itemize}[leftmargin=1.3em,itemsep=2pt,topsep=2pt]
\item \textbf{Balanced Accuracy = 0.6365}:
  \begin{itemize}[leftmargin=1.3em,itemsep=2pt,topsep=2pt]
  \item Macro recall \textasciitilde{}0.64 across six classes indicates the model captures a substantial portion of each class's events, despite heavy imbalance and noisy clinical data.
  \item This is a strong result relative to earlier baselines in the same pipeline, where many variants yielded balanced accuracies around 0.45--0.58.

  \end{itemize}
\item \textbf{Cohen's Kappa = 0.3491}:
  \begin{itemize}[leftmargin=1.3em,itemsep=2pt,topsep=2pt]
  \item Indicates \textbf{moderate agreement} beyond chance.
  \item The gap between $\kappa$ and Balanced Accuracy suggests that while the classifier has reasonable per-class recall, confusion among classes (especially among non-background events) still limits overall agreement.

  \end{itemize}
\item \textbf{Weighted F1 = 0.6122}:
  \begin{itemize}[leftmargin=1.3em,itemsep=2pt,topsep=2pt]
  \item Reflects performance weighted by class frequency.
  \item The value is close to the balanced accuracy, indicating that improvements are not driven solely by dominant classes; minority event types also benefit from the deeper model and training strategy.

  \end{itemize}
\end{itemize}

\smallskip\noindent\textit{Contribution of design choices}\par

Within the fixed preprocessing and splitting protocol, the key improvements reflected in these metrics are:

\begin{enumerate}[leftmargin=1.5em,itemsep=2pt,topsep=2pt]
\item \textbf{Multi-scale temporal modeling}:
  \begin{itemize}[leftmargin=1.3em,itemsep=2pt,topsep=2pt]
  \item A 4-block 1D ResNet with internal pooling at every stage progressively halves the temporal resolution, providing four scales of context within the 5-second window without inflating model depth.

  \end{itemize}
\item \textbf{Combination of imbalance-aware strategies}:
  \begin{itemize}[leftmargin=1.3em,itemsep=2pt,topsep=2pt]
  \item Class-weighted cross-entropy combined with \texttt{WeightedRandomSampler} mitigates the severe skew towards background/artifact events at both the loss and the batch-sampling level.
  \item Temporal jitter improves robustness to labeling jitter and slight misalignment of events.

  \end{itemize}
\item \textbf{Stabilized optimization}:
  \begin{itemize}[leftmargin=1.3em,itemsep=2pt,topsep=2pt]
  \item Cosine-annealing with warm restarts provides a smooth training trajectory with periodic exploration, avoiding overfitting at high LR and underfitting from overly aggressive decay.

  \end{itemize}
\end{enumerate}
Overall, the final metrics indicate that the chosen configuration successfully balances capacity, regularization, and imbalance handling to achieve strong macro recall on this difficult 6-class clinical EEG benchmark.

\noindent\rule{\linewidth}{0.3pt}

\smallskip\noindent\textbf{Future Work}\par

Potential directions to further improve performance and robustness include:

\begin{enumerate}[leftmargin=1.5em,itemsep=2pt,topsep=2pt]
\item \textbf{Class-specific calibration and thresholds}
  \begin{itemize}[leftmargin=1.3em,itemsep=2pt,topsep=2pt]
  \item Analyze per-class precision-recall and confusion patterns to tune decision thresholds or incorporate cost-sensitive decision rules, especially for rare seizure-related classes (spsw, gped, pled).

  \end{itemize}
\item \textbf{Per-channel and spatial modeling}
  \begin{itemize}[leftmargin=1.3em,itemsep=2pt,topsep=2pt]
  \item Introduce spatial attention or depthwise spatial convolutions to better exploit inter-electrode relationships, possibly combined with learnable montages.
  \item Investigate learnable channel embeddings that respect known neurophysiological topology.

  \end{itemize}
\item \textbf{Sequence-level aggregation}
  \begin{itemize}[leftmargin=1.3em,itemsep=2pt,topsep=2pt]
  \item Current pipeline classifies isolated 5 s segments. Sequence models (e.g., temporal pooling, transformers, or recurrent layers over consecutive windows) may capture contextual evolution of events across time, improving difficult distinctions.

  \end{itemize}
\item \textbf{More targeted augmentation}
  \begin{itemize}[leftmargin=1.3em,itemsep=2pt,topsep=2pt]
  \item Explore physiologically informed augmentations (e.g., amplitude scaling within safety bounds, narrowband noise consistent with recording artifacts) beyond simple temporal jitter.
  \item Consider per-class or per-channel augmentation policies (e.g., less aggressive mixing for rare epileptiform events).

  \end{itemize}
\item \textbf{Curriculum and hard-example mining}
  \begin{itemize}[leftmargin=1.3em,itemsep=2pt,topsep=2pt]
  \item Progressive training that starts on more frequent/clear examples and gradually emphasizes rare or ambiguous events.
  \item Online hard example mining or focal-style weighting at the sample level, but carefully tuned to avoid instability observed in some focal-loss experiments.

  \end{itemize}
\item \textbf{Model ensembling}
  \begin{itemize}[leftmargin=1.3em,itemsep=2pt,topsep=2pt]
  \item Combine several high-performing runs (e.g., different random seeds or slight architectural variants) via probability averaging to reduce variance and improve robustness, particularly on the minority classes.

  \end{itemize}
\item \textbf{Domain adaptation and calibration}
  \begin{itemize}[leftmargin=1.3em,itemsep=2pt,topsep=2pt]
  \item Investigate calibration methods (e.g., temperature scaling) and domain adaptation to reduce potential shift between training and \texttt{/eval} recordings.
  \item Evaluate reliability of predicted probabilities for downstream clinical decision support.

  \end{itemize}
\end{enumerate}
These directions build directly on the current best pipeline and are compatible with the strict preprocessing and data-splitting constraints imposed by the TUEV benchmark.
\end{neuroweaverreport}
\clearpage
