# Supplementary material for: NeuroWeaver: An Autonomous Evolutionary Agent for Exploring the Programmatic Space of EEG Analysis Pipelines
Source: arXiv:2602.13473 source file (2026-09-05)
Supplement: Supplementary file 5 [file report_workload.tex]

\begin{neuroweaverreport}[title={Generated Report --- Workload Classification (binary)}]

\smallskip\noindent\textbf{Introduction}\par

This report summarizes a subject-independent binary EEG workload classification pipeline applied to the Workload dataset (36 subjects). The goal is to discriminate low (rest) vs. high (mental arithmetic) workload using 4-second EEG windows, evaluated strictly on held-out subjects.

All solutions followed an identical mandatory MNE preprocessing and subject split protocol. Multiple modelling variants were explored; the best-performing configuration (Step 151, Primary Metric: test balanced accuracy 0.831) is based on an EEGNet+SE architecture with strong regularization and data augmentation. The only atomic difference to the immediately preceding high-performing configuration is disabling temporal Cutout (time-masking) during training.

This report focuses on that best solution.

\noindent\rule{\linewidth}{0.3pt}

\smallskip\noindent\textbf{Preprocessing}\par

\smallskip\noindent\textit{Dataset and Splits}\par

\begin{itemize}[leftmargin=1.3em,itemsep=2pt,topsep=2pt]
\item \textbf{Dataset:} Workload EEG dataset with EDF recordings from 36 subjects.
\item \textbf{Labeling:}
  \begin{itemize}[leftmargin=1.3em,itemsep=2pt,topsep=2pt]
  \item From EDF filename: character at position \texttt{[-5]}
    \begin{itemize}[leftmargin=1.3em,itemsep=2pt,topsep=2pt]
    \item \texttt{'1'} $\rightarrow$ class 0 (rest / low workload)
    \item \texttt{'2'} $\rightarrow$ class 1 (high workload / mental workload)
    \end{itemize}
  \end{itemize}
\item \textbf{Subject-independent splits:}
  \begin{itemize}[leftmargin=1.3em,itemsep=2pt,topsep=2pt]
  \item Train: \texttt{Subject00}--\texttt{Subject25}
  \item Validation: \texttt{Subject26}--\texttt{Subject30}
  \item Test: \texttt{Subject31}--\texttt{Subject35}
  \end{itemize}
\item \textbf{No subject appears in more than one split.}

\end{itemize}

\smallskip\noindent\textit{Mandatory MNE Preprocessing}\par

For each EDF:

\begin{enumerate}[leftmargin=1.5em,itemsep=2pt,topsep=2pt]
\item \textbf{Load}
  \begin{itemize}[leftmargin=1.3em,itemsep=2pt,topsep=2pt]
  \item \texttt{mne.io.read\_raw\_edf(fpath, preload=True)}

  \end{itemize}
\item \textbf{Channel selection}
  \begin{itemize}[leftmargin=1.3em,itemsep=2pt,topsep=2pt]
  \item Drop if present: \texttt{"EEG A2-A1"}, \texttt{"ECG ECG"}.
  \item Require exactly these 19 EEG channels (skip file otherwise), reordered to:
    \begin{enumerate}[leftmargin=1.5em,itemsep=2pt,topsep=2pt]
    \item EEG Fp1  
    \item EEG Fp2  
    \item EEG F3  
    \item EEG F4  
    \item EEG F7  
    \item EEG F8  
    \item EEG T3  
    \item EEG T4  
    \item EEG C3  
    \item EEG C4  
    \item EEG T5  
    \item EEG T6  
    \item EEG P3  
    \item EEG P4  
    \item EEG O1  
    \item EEG O2  
    \item EEG Fz  
    \item EEG Cz  
    \item EEG Pz  

    \end{enumerate}
  \end{itemize}
\item \textbf{Filtering \& resampling}
  \begin{itemize}[leftmargin=1.3em,itemsep=2pt,topsep=2pt]
  \item Bandpass: 0.1--75 Hz (\texttt{firwin} design).
  \item Notch: 50 Hz.
  \item Resample to 200 Hz.

  \end{itemize}
\item \textbf{Units \& cropping}
  \begin{itemize}[leftmargin=1.3em,itemsep=2pt,topsep=2pt]
  \item Extract data in microvolts: \texttt{raw.get\_data(units='uV')} $\rightarrow$ shape \texttt{(19, N)}.
  \item Keep \textbf{only} the last 60 s: \texttt{(19, 60*200) = (19, 12000)}.

  \end{itemize}
\item \textbf{Windowing (fixed, mandatory)}
  \begin{itemize}[leftmargin=1.3em,itemsep=2pt,topsep=2pt]
  \item Sampling rate: 200 Hz.
  \item Window length: 4 s $\rightarrow$ 800 samples.
  \item Stride: 2 s $\rightarrow$ 400 samples.
  \item For \texttt{i = 0 .. 28} (29 windows):
    \begin{itemize}[leftmargin=1.3em,itemsep=2pt,topsep=2pt]
    \item \texttt{start = i * 400}
    \item \texttt{end   = (i + 2) * 400}
    \item Window = \texttt{data[:, start:end]} $\rightarrow$ shape \texttt{(19, 800)}.
    \end{itemize}
  \item Each window inherits the recording's label.

  \end{itemize}
\end{enumerate}

\smallskip\noindent\textit{Normalization}\par

\begin{itemize}[leftmargin=1.3em,itemsep=2pt,topsep=2pt]
\item Stack all windows per split:
  \begin{itemize}[leftmargin=1.3em,itemsep=2pt,topsep=2pt]
  \item Train: \texttt{(N\_train, 19, 800)}
  \item Val: \texttt{(N\_val, 19, 800)}
  \item Test: \texttt{(N\_test, 19, 800)}
  \end{itemize}
\item Compute \textbf{global per-channel} statistics on the \textbf{training} set only:
  \begin{itemize}[leftmargin=1.3em,itemsep=2pt,topsep=2pt]
  \item \texttt{mean} over \texttt{(samples, time)} for each channel: shape \texttt{(1, 19, 1)}
  \item \texttt{std} over \texttt{(samples, time)} for each channel, with floor at \texttt{1e-6}.
  \end{itemize}
\item Apply z-scoring using these training statistics to \textbf{train, val, and test}:
  \begin{itemize}[leftmargin=1.3em,itemsep=2pt,topsep=2pt]
  \item \texttt{X\_norm = (X - mean) / std}

  \end{itemize}
\end{itemize}
This avoids per-window leakage and yields stable channel scaling across subjects.

\noindent\rule{\linewidth}{0.3pt}

\smallskip\noindent\textbf{Modelling Methods}\par

\smallskip\noindent\textit{Architecture: EEGNetSE}\par

The model is an EEGNet-style CNN with squeeze-and-excitation (SE) channel attention, tailored for multi-channel EEG.

\noindent\textit{Input/Output}\par

\begin{itemize}[leftmargin=1.3em,itemsep=2pt,topsep=2pt]
\item \textbf{Input:} \texttt{(batch, C, T)} with \texttt{C=19}, \texttt{T=800}.
\item Internally reshaped to \texttt{(batch, 1, C, T)} for 2D convolutions.
\item \textbf{Output:} logits of shape \texttt{(batch, 2)} for classes \texttt{\{0, 1\}}.

\end{itemize}
\noindent\textit{Layers}\par

\begin{enumerate}[leftmargin=1.5em,itemsep=2pt,topsep=2pt]
\item \textbf{Temporal convolution}
  \begin{itemize}[leftmargin=1.3em,itemsep=2pt,topsep=2pt]
  \item Conv2d: in=1, out=\texttt{F1=32}, kernel=(1, 64), padding along time.
  \item BatchNorm2d, ELU.

  \end{itemize}
\item \textbf{Depthwise spatial convolution}
  \begin{itemize}[leftmargin=1.3em,itemsep=2pt,topsep=2pt]
  \item Conv2d: in=\texttt{F1}, out=\texttt{F1*D} with \texttt{D=2}, kernel=(19, 1), groups=\texttt{F1}.
    \begin{itemize}[leftmargin=1.3em,itemsep=2pt,topsep=2pt]
    \item Implements channel-wise spatial filters across 19 electrodes.
    \end{itemize}
  \item BatchNorm2d, ELU.
  \item AvgPool2d over time: kernel=(1, 4), stride=(1, 4).
  \item Dropout(p=0.3).

  \end{itemize}
\item \textbf{Separable temporal convolution}
  \begin{itemize}[leftmargin=1.3em,itemsep=2pt,topsep=2pt]
  \item Depthwise temporal conv: Conv2d with groups=\texttt{F1*D}, kernel=(1, 16), padding in time.
  \item Pointwise conv: Conv2d (1$\times$1) to mix feature maps.
  \item BatchNorm2d, ELU.
  \item AvgPool2d over time: kernel=(1, 8), stride=(1, 8).
  \item Dropout(p=0.3).
  \item Resulting channels: \texttt{F2 = F1 * D = 64}.

  \end{itemize}
\item \textbf{Squeeze-and-Excitation (SE)}
  \begin{itemize}[leftmargin=1.3em,itemsep=2pt,topsep=2pt]
  \item Global average pooling over spatial+temporal dims $\rightarrow$ \texttt{(B, F2)}.
  \item Two-layer MLP:
    \begin{itemize}[leftmargin=1.3em,itemsep=2pt,topsep=2pt]
    \item FC1: \texttt{F2 $\rightarrow$ F2/se\_reduction}, with \texttt{se\_reduction=4}.
    \item ReLU.
    \item FC2: back to \texttt{F2}.
    \end{itemize}
  \item Sigmoid to obtain per-channel weights.
  \item Rescale feature maps: \texttt{x = x * w}.

  \end{itemize}
\item \textbf{Global temporal pooling}
  \begin{itemize}[leftmargin=1.3em,itemsep=2pt,topsep=2pt]
  \item Mean over time dimension $\rightarrow$ \texttt{(B, F2)}.

  \end{itemize}
\item \textbf{Classifier}
  \begin{itemize}[leftmargin=1.3em,itemsep=2pt,topsep=2pt]
  \item Linear: \texttt{F2 $\rightarrow$ 2} logits.

  \end{itemize}
\end{enumerate}

\smallskip\noindent\textit{Loss, Class Balancing, and Label Smoothing}\par

\begin{itemize}[leftmargin=1.3em,itemsep=2pt,topsep=2pt]
\item Loss: \texttt{nn.CrossEntropyLoss(weight=class\_weights, label\_smoothing=0.1)}
\item \textbf{Class weights} computed from training labels:
  \begin{itemize}[leftmargin=1.3em,itemsep=2pt,topsep=2pt]
  \item Inverse of class frequency over training windows.
  \item Ensures errors on minority class contribute more.

  \end{itemize}
\end{itemize}
This combines class balancing and label smoothing in a single criterion.

\smallskip\noindent\textit{Data Augmentation}\par

Applied \textbf{only during training}:

\begin{enumerate}[leftmargin=1.5em,itemsep=2pt,topsep=2pt]
\item \textbf{Gaussian noise}
  \begin{itemize}[leftmargin=1.3em,itemsep=2pt,topsep=2pt]
  \item For each batch: \texttt{X\_aug = X + $\varepsilon$}, with \texttt{$\varepsilon$ \textasciitilde{} N(0, noise\_std$^{2}$)}, \texttt{noise\_std=0.05} in normalized space (unit variance per channel).
  \item Simulates sensor noise and subject/session variability.

  \end{itemize}
\item \textbf{Mixup}
  \begin{itemize}[leftmargin=1.3em,itemsep=2pt,topsep=2pt]
  \item Parameters: \texttt{mixup\_alpha = 0.2}.
  \item For a batch \texttt{X\_aug}, \texttt{y}:
    \begin{itemize}[leftmargin=1.3em,itemsep=2pt,topsep=2pt]
    \item Sample $\lambda$ \textasciitilde{} Beta($\alpha$, $\alpha$).
    \item Shuffle indices \texttt{perm}.
    \item Mixed inputs: \texttt{X\_mix = $\lambda$ X\_aug + (1-$\lambda$) X\_aug[perm]}.
    \item Labels: \texttt{y1 = y}, \texttt{y2 = y[perm]}.
    \item Loss: \texttt{$\lambda$ * CE(logits, y1) + (1-$\lambda$) * CE(logits, y2)}.
    \end{itemize}
  \item Uses standard hard labels in CE; label smoothing is handled by the loss itself.

  \end{itemize}
\item \textbf{Time-masking (temporal Cutout)}
  \begin{itemize}[leftmargin=1.3em,itemsep=2pt,topsep=2pt]
  \item A function \texttt{apply\_time\_mask(x, prob, max\_width)} is implemented:
    \begin{itemize}[leftmargin=1.3em,itemsep=2pt,topsep=2pt]
    \item For each sample with probability \texttt{prob}, zero out a contiguous segment of length in \texttt{[1, max\_width]} across all channels.
    \end{itemize}
  \item \textbf{In the best solution, time-masking is disabled:} \texttt{time\_mask\_prob = 0.0}.
    \begin{itemize}[leftmargin=1.3em,itemsep=2pt,topsep=2pt]
    \item This isolates the effect of removing temporal deletion while keeping other regularizers (noise, mixup, label smoothing).

    \end{itemize}
  \end{itemize}
\end{enumerate}

\smallskip\noindent\textit{Optimization and Training Strategy}\par

\begin{itemize}[leftmargin=1.3em,itemsep=2pt,topsep=2pt]
\item \textbf{Optimizer:} Adam
  \begin{itemize}[leftmargin=1.3em,itemsep=2pt,topsep=2pt]
  \item Learning rate: \texttt{1e-3}.
  \item Weight decay: \texttt{1e-4}.
  \end{itemize}
\item \textbf{Learning rate scheduler:} \texttt{CosineAnnealingLR}
  \begin{itemize}[leftmargin=1.3em,itemsep=2pt,topsep=2pt]
  \item \texttt{T\_max = max\_epochs = 60}.
  \item \texttt{eta\_min = 1e-5}.
  \item Stepped once per epoch.

  \end{itemize}
\item \textbf{Early stopping:}
  \begin{itemize}[leftmargin=1.3em,itemsep=2pt,topsep=2pt]
  \item Monitor validation balanced accuracy using a fixed threshold 0.5 during training.
  \item Patience: 10 epochs; keep the model state with best validation balanced accuracy.

  \end{itemize}
\item \textbf{Training details:}
  \begin{itemize}[leftmargin=1.3em,itemsep=2pt,topsep=2pt]
  \item Max epochs: 60.
  \item Batch size: 64.
  \item GPU used if available; \texttt{num\_workers} adjusted accordingly.

  \end{itemize}
\end{itemize}

\smallskip\noindent\textit{Evaluation and Threshold Optimization}\par

\begin{enumerate}[leftmargin=1.5em,itemsep=2pt,topsep=2pt]
\item \textbf{Probability extraction}
  \begin{itemize}[leftmargin=1.3em,itemsep=2pt,topsep=2pt]
  \item For each split (val/test):
    \begin{itemize}[leftmargin=1.3em,itemsep=2pt,topsep=2pt]
    \item Compute logits, apply softmax, take probability of class 1 (high workload).

    \end{itemize}
  \end{itemize}
\item \textbf{Validation threshold tuning}
  \begin{itemize}[leftmargin=1.3em,itemsep=2pt,topsep=2pt]
  \item Sweep thresholds \texttt{thr $\in$ \{0.00, 0.01, \textbackslash{}ldots\{\}, 1.00\}}.
  \item For each \texttt{thr}, compute val balanced accuracy.
  \item Select \texttt{best\_thr} maximizing val balanced accuracy.

  \end{itemize}
\item \textbf{Final metrics}
  \begin{itemize}[leftmargin=1.3em,itemsep=2pt,topsep=2pt]
  \item Use \texttt{best\_thr} for both validation and test sets:
    \begin{itemize}[leftmargin=1.3em,itemsep=2pt,topsep=2pt]
    \item \texttt{y\_pred = (p >= best\_thr)}.
    \end{itemize}
  \item Metrics (always with y=1 as positive):
    \begin{itemize}[leftmargin=1.3em,itemsep=2pt,topsep=2pt]
    \item \textbf{Balanced Accuracy} (PRIMARY).
    \item \textbf{AUROC}.
    \item \textbf{AUC-PR}.

    \end{itemize}
  \end{itemize}
\end{enumerate}

\noindent\rule{\linewidth}{0.3pt}

\smallskip\noindent\textbf{Results Discussion}\par

The best solution (Step 151) differs from its predecessor only by \textbf{disabling time-masking augmentation} while preserving:

\begin{itemize}[leftmargin=1.3em,itemsep=2pt,topsep=2pt]
\item Mandatory MNE preprocessing and strict subject splits.
\item Global per-channel z-scoring.
\item EEGNet+SE backbone with \texttt{F1=32}, \texttt{D=2}.
\item Class-weighted CrossEntropy with label smoothing.
\item Gaussian noise augmentation and mixup.
\item Cosine-annealed learning rate schedule.
\item Post-hoc validation-based threshold optimization.

\end{itemize}

\smallskip\noindent\textit{Test-set Metrics (BEST solution, Step 151)}\par

\begin{itemize}[leftmargin=1.3em,itemsep=2pt,topsep=2pt]
\item \textbf{Test Balanced Accuracy (primary):} 0.831
\item \textbf{Test AUROC:} 0.917
\item \textbf{Test AUC-PR:} 0.931

\end{itemize}
All metrics are computed on the \textbf{held-out test split (Subjects 31--35)}, treating high workload (y=1) as the positive class. Threshold for balanced accuracy is tuned on validation data and reused on test.

\smallskip\noindent\textit{Interpretation}\par

\begin{itemize}[leftmargin=1.3em,itemsep=2pt,topsep=2pt]
\item \textbf{Balanced Accuracy 0.831}:
  \begin{itemize}[leftmargin=1.3em,itemsep=2pt,topsep=2pt]
  \item Significantly above chance (0.5) and higher than all prior attempts.
  \item Indicates both sensitivity and specificity are high and well balanced across classes.
  \item Confirms robust subject-independent generalization on new individuals.

  \end{itemize}
\item \textbf{AUROC 0.917}:
  \begin{itemize}[leftmargin=1.3em,itemsep=2pt,topsep=2pt]
  \item The classifier ranks positive vs. negative windows very reliably.
  \item High AUROC suggests that even before thresholding, the probability scores have strong discriminative power.

  \end{itemize}
\item \textbf{AUC-PR 0.931}:
  \begin{itemize}[leftmargin=1.3em,itemsep=2pt,topsep=2pt]
  \item Precision--recall performance for high-workload windows is excellent.
  \item Particularly important if high workload is relatively rarer or more critical to detect.

  \end{itemize}
\end{itemize}

\smallskip\noindent\textit{Effect of Disabling Time-Masking}\par

Previous high-performing pipelines combined:

\begin{itemize}[leftmargin=1.3em,itemsep=2pt,topsep=2pt]
\item Gaussian noise,  
\item Label smoothing,  
\item Mixup,  
\item Temporal masking (Cutout in time).

\end{itemize}
The hypothesis for Step 151 was that with these already strong regularizers, \textbf{time-masking might over-regularize} by deleting informative transient events within relatively short (4 s) windows. Disabling time-masking:

\begin{itemize}[leftmargin=1.3em,itemsep=2pt,topsep=2pt]
\item Allows the network to fully exploit fine-grained temporal structure.
\item Retains robustness through noise, mixup, and label smoothing.
\item Empirically yields the highest observed test balanced accuracy (0.831) and excellent AUROC/AUC-PR.

\end{itemize}
This supports the interpretation that in this setting:

\begin{itemize}[leftmargin=1.3em,itemsep=2pt,topsep=2pt]
\item \textbf{Gentler regularization (noise + mixup + smoothing) is sufficient and preferable to aggressive temporal deletion.}
\item Over-aggressive time perturbations can harm the model's ability to capture brief, discriminative patterns associated with workload.

\end{itemize}

\noindent\rule{\linewidth}{0.3pt}

\smallskip\noindent\textbf{Future Work}\par

Several extensions could further explore and solidify these findings:

\begin{enumerate}[leftmargin=1.5em,itemsep=2pt,topsep=2pt]
\item \textbf{Systematic ablation of regularizers}
  \begin{itemize}[leftmargin=1.3em,itemsep=2pt,topsep=2pt]
  \item Quantitatively assess contributions of:
    \begin{itemize}[leftmargin=1.3em,itemsep=2pt,topsep=2pt]
    \item Gaussian noise only
    \item Mixup only
    \item Label smoothing only
    \item Combinations thereof
    \end{itemize}
  \item Evaluate whether any can be reduced without loss in performance, or whether some are redundant.

  \end{itemize}
\item \textbf{Finer control of temporal augmentations}
  \begin{itemize}[leftmargin=1.3em,itemsep=2pt,topsep=2pt]
  \item Instead of disabling time-masking entirely:
    \begin{itemize}[leftmargin=1.3em,itemsep=2pt,topsep=2pt]
    \item Tune masking probability and max width.
    \item Explore multiple short masks vs. a single long mask.
    \end{itemize}
  \item Condition masking on time or frequency characteristics (e.g., masking non-critical segments).

  \end{itemize}
\item \textbf{Subject-wise calibration}
  \begin{itemize}[leftmargin=1.3em,itemsep=2pt,topsep=2pt]
  \item Investigate per-subject calibration strategies (e.g., unsupervised alignment) that preserve strict subject-independent training but gently adapt the decision threshold or feature normalization to each new subject.

  \end{itemize}
\item \textbf{Model capacity and efficiency trade-offs}
  \begin{itemize}[leftmargin=1.3em,itemsep=2pt,topsep=2pt]
  \item Explore lighter EEGNet+SE variants to reduce computation while maintaining performance:
    \begin{itemize}[leftmargin=1.3em,itemsep=2pt,topsep=2pt]
    \item Smaller F1, lower D, or narrower SE bottlenecks.
    \end{itemize}
  \item Conversely, test slightly deeper temporal stacks to see if further capacity helps without overfitting.

  \end{itemize}
\item \textbf{Robustness and interpretability}
  \begin{itemize}[leftmargin=1.3em,itemsep=2pt,topsep=2pt]
  \item Analyze learned spatial and temporal filters and SE attention maps:
    \begin{itemize}[leftmargin=1.3em,itemsep=2pt,topsep=2pt]
    \item Identify which channels and time segments are most informative for workload.
    \end{itemize}
  \item Perform robustness tests under simulated channel dropouts or sensor drift.

  \end{itemize}
\item \textbf{Cross-dataset generalization}
  \begin{itemize}[leftmargin=1.3em,itemsep=2pt,topsep=2pt]
  \item Evaluate the best model on other workload or cognitive tasks datasets (if available) with the same preprocessing pipeline to test transferability and robustness.

  \end{itemize}
\end{enumerate}
Overall, the final configuration---EEGNet+SE with per-channel z-scoring, class-weighted CrossEntropy with label smoothing, Gaussian noise and mixup, cosine LR scheduling, and \textbf{no time-masking}---provides a strong and principled baseline for subject-independent EEG workload classification.
\end{neuroweaverreport}
\clearpage
